# Supplementary material for: Uncertainty-Resilient Multimodal Learning via Consistency-Guided Cross-Modal Transfer
Source: arXiv:2511.15741 source file (2025-11-18)
Supplement: Supplementary file 1 [file appendices.tex]

% \input{chapters/appendix_codes}
